# Supplementary material for: Coding Agents Are Zero-Shot Coordinators
Source: arXiv:2611.37528 source file (2026-11-27)
Supplement: Supplementary file 1 [file appendix_contents.tex]

\section*{Appendix}
\makeatletter
\begingroup
  \hypersetup{linkcolor=black,linktoc=all}
  \c@tocdepth=2\relax
  \renewcommand*{\l@section}[2]{%
    \par\addvspace{.45em}%
    {\bfseries\setlength{\@tempdima}{1.65em}%
     \noindent#1\hfill\mbox{#2}\par}}
  \renewcommand*{\l@subsection}{\@dottedtocline{2}{.8em}{2.4em}}
  \begin{tcolorbox}[
    title={Table of Contents},fonttitle=\bfseries,
    colback=white,colframe=black!35,colbacktitle=black!35,coltitle=white,
    sharp corners,boxrule=.5pt,boxsep=0pt,
    left=12pt,right=12pt,top=5pt,bottom=8pt,toptitle=3pt,bottomtitle=3pt]
    \small\@starttoc{atoc}
  \end{tcolorbox}
\endgroup
\let\appendixOriginalContentsLine\addcontentsline
\ExplSyntaxOn
\renewcommand{\addcontentsline}[3]{
  \str_if_eq:nnT {#1} {toc} {
    \addtocontents{atoc}{\protect\contentsline{#2}{#3}{\thepage}{\@currentHref}}
  }
  \appendixOriginalContentsLine{#1}{#2}{#3}
}
\ExplSyntaxOff
\makeatother
\clearpage
